# Supplementary material for: Green Operations of SWIPT Networks: The Role of End-User Devices
Source: arXiv:2312.08232 source file (2024-10-31)
Supplement: Supplementary file 1 [file Appendix_long.tex]

\appendix

\subsection{Proof of \thref{th:BE_tau} (sketch)}
\label{app:proof_th_BE_tau}
Here we sketch the main steps of the derivation while for the full proof we refer to the extended version \cite{XXX}. The derivation of the expression of the per-bit delay goes along the same lines as the proof of Theorem $3.1$ in \cite{rengarajan2015energy}. The main variants are the use of the palm expectation of $I(r,k)$,  $\bar{I}(r,k,\bar{\tau})$, instead of $I(r,k)$, in order to make the derivation analytically tractable.

\begin{lemma} For $p\leq 20 W$, and $\lambda_b\leq 0.01$ $BS/m^2$, the fixed point in \thref{th:BE_tau} admits a unique solution.
\end{lemma}
%\textbf{(raffina: rendi piu' formale. Spiega a cosa e' dovuta la dip dai parametri)}
\begin{proof}%[Uniqueness of solution of fixed point problem \eref{eq:Poisson}]
In order to prove that \eref{eq:Poisson} has a unique fixed point, we have to prove that the operator 
$T(\bar{\tau})$, whose expression is given by the right member of \eref{eq:Poisson}, is a contraction. To do so, we verify that Blackwell's sufficient conditions for a contraction \cite{blackwell1965discounted} hold for $T$. The monotonicity of $T$ is straightforward, as with increasing $\bar{\tau}$ increases the mean BS  utilization, and hence their interference. And this translates into an increase in per-bit delays computed in \eref{eq:Poisson}.\\
For the discounting property, we have to prove that $\exists \beta\in(0,1)$ such that $T(\bar{\tau}+ a)\leq T(\bar{\tau})+\beta a$, $\forall a \geq 0$ and for all system parameter values for which  
$\bar{\tau}$ is defined. We have $U(\bar{\tau}+ a)=U(\bar{\tau})+Ka$, with 
\[
K=\frac{\left[1+\gamma\left(R_{0}\frac{\mu_H^{-1}}{\mu_H^{-1}+\mu_W^{-1}}\bar{\tau}^{0}-1\right)\right]}{\bar{\tau}^{0}} 
\]
Substituting into the capacity formula \ref{eq:capacity}, we have 
\[
C(r,\bar{\tau}+a) = 
\]

\[
=(B/k) \log_{2}\left(1 + \frac{p r^{-\alpha}}{N_0+I(r,k)+K a p r^{-\alpha}}\right)=
\]

\[
=(B/k) \log_{2}\left(N_0+I(r,k)+K a p r^{-\alpha} + p r^{-\alpha}\right)+
\]
\[
-(B/k)\log_{2}\left(N_0+I(r,k)+K a p r^{-\alpha} \right)\geq
\]

\[
\geq (B/k) \log_{2}\left(N_0+I(r,k)+K a p r^{-\alpha} + p r^{-\alpha}\right)+
\]
\[
-(B/k)\log_{2}\left(N_0+I(r,k)\right)-(B/k)\log_{2}\left(K a p r^{-\alpha} \right)
\]

\[
\geq (B/k)\left[ \log_{2}\left(1 + \frac{p r^{-\alpha}(1+Ka)}{N_0+I(r,k)}\right)-\log_{2}\left(K a p r^{-\alpha} \right)\right]
\]
as $Ka\geq 0$,
\[
\geq (B/k)\left[ \log_{2}\left(1 + \frac{p r^{-\alpha}}{N_0+I(r,k)}\right)-\log_{2}\left(K a p r^{-\alpha} \right)\right]
\]
Then we can write
\[T(\bar{\tau}+ a)\leq \]
\[\leq\int_0^{\infty} \left(\int_0^{\infty} \int_0^{2 \pi} 
e^{- \lambda_b A(r, x, \theta)} \lambda_{u} x \diff\theta \diff x  \right)\cdot
\]
\[
\cdot\frac{e^{- \lambda_b \pi r^2} \lambda_b 2 \pi r}{C(r,\bar{\tau})-(B/k)\log_{2}\left(K a p r^{-\alpha}\right)} \diff r
\]
We apply the Taylor series expansion of $\frac{1}{c-x}$ for $x\rightarrow 0$ to the fraction at the integrand, and we have, for $a \rightarrow 0$

\[
\frac{1}{C(r,\bar{\tau})-(B/k)\log_{2}\left(K a p r^{-\alpha}\right)}\geq
\] 

\[
\geq \frac{1}{C(r,\bar{\tau})}+(B/k)\frac{\log_{2}\left(K a p r^{-\alpha}\right)}{C^2(r,\bar{\tau})}
\]
%To prove the discounting property, we have to prove that 
Now we have 
\[
(B/k)\frac{\log_{2}\left(K a p r^{-\alpha}\right)}{C(r,\bar{\tau})}=
\]

\[
\frac{\log_{2}\left(K a p r^{-\alpha}\right)}{log_{2}\left(1 + \frac{p r^{-\alpha}}{N_0+I(r,k)}\right)}\leq
\]
\be\label{eq:inequality1}
\leq K a\frac{\log_{2}\left( p r^{-\alpha}\right)}{log_{2}\left(1 + \frac{p r^{-\alpha}}{N_0+I(r,k)}\right)}
\ee

By substituting the expression in \eref{eq:interference} for the interfering power, we can easily see that if system parameter values are within the typical range for a small cell RAN ($p\leq 20 W$, and $\lambda_b\leq 0.01$ $BS/m^2$), we can write 

\[
\frac{\log_{2}\left( p r^{-\alpha}\right)}{log_{2}\left(1 + \frac{p r^{-\alpha}}{N_0+I(r,k)}\right)}\leq \beta
\]
with $0\leq \beta <1$. Hence we have 
\[
\leq K\beta a
\]
 
Putting all together, we have

 \[
T(\bar{\tau}+ a)\leq T(\bar{\tau}) (1 + K \beta a)=
\]

\[ = T(\bar{\tau}) + a\beta\left[1+\gamma\left(R_{0}\frac{\mu_H^{-1}}{\mu_H^{-1}+\mu_W^{-1}}\bar{\tau}^{0}-1\right)\right] \frac{T(\bar{\tau})}{T_{0}}
\]
and as the utilization $U\leq 1$
\[
\leq T(\bar{\tau}) + \beta a 
\]
which proves the discounting property.\\
Being $T(\bar{\tau})$ a contraction, by the Banach fixed point theorem, the fixed point problem in \eref{eq:Poisson} admits a unique solution.
\end{proof}
